# Supplementary material for: DRILL-- Deep Reinforcement Learning for Refinement Operators in $\mathcal{ALC}$
Source: arXiv:2106.15373 source file (2021-06-29)
Supplement: Supplementary file 1 [file supplemental.tex]

\section{Supplementary Material}

\subsection{Quality of Concept}
The F-measure of a node w.r.t. $E^+$ and $E^-$ calculated composition of as the Precision and Recall of a node as follows

\begin{equation}
    \text{F-measure}(s)= 2 \times \Bigg( \frac{\text{Precision}(s) \times \text{Recall}(s)}{\text{Precision}(s) + \text{Recall}(s)} \Bigg).
    \label{f_measure}
\end{equation}

\begin{equation}
    \text{Precision}(s)=\frac{|E^+ \cap \retriever(s)|}{|E^+ \cap \retriever(s)| +|E^- \cap \retriever(s)| }.
    \label{precision}
\end{equation}

\begin{equation}
    \text{Recall}(s)=\frac{|E^+ \cap \retriever(s)|}{|E^+ \cap \retriever(s)| +|E^+ \setminus \retriever(s)| }.
    \label{recall}
\end{equation} where the retrieval function $\retriever:\SearchSpace \mapsto \Objects$ is a mapping from concepts to a set of individuals that belongs to a given concept~\cite{lehmann2010concept}.
